# Supplementary material for: TreeCaps: Tree-Based Capsule Networks for Source Code Processing
Source: arXiv:2009.09777 source file (2020-12-14)
Supplement: Supplementary file 1 [file supplementary.tex]

\subsubsection{Effect of the variable-to-static routing algorithm}
We investigate the effect of the variable-to-static routing algorithm by replacing it with Dynamic Max Pooling (DMP). We use the program classification task for this investigation. Since there is no alternative approach existing in the literature for routing a variable set of capsules to a static set of capsules, we compare the proposed routing algorithm with dynamic pooling. The output of the PVC layer, $\mathbf{X_{pvc}}\in \mathbb{R}^{N_{pvc}\times D_{pvc}}$ consists of a variable component, $N_{pvc}$. Using dynamic max-pooling across all the $N_{pvc}$ capsules will result in one output capsule, $\mathbf{X_{dmp}}\in \mathbb{R}^{1\times D_{pvc}}$. Since $\mathbf{X_{dmp}}$ has no variable components across the training samples, it can now be routed to the code capsules using the dynamic routing algorithm. However, it should be noted that DMP is not suitable for capsule networks, as it destroys the spatial and dependency relationships between the capsules. We use DMP here only for comparison purposes.

As summarized in Table \ref{tab:ablation}, DMP yields a considerably lower accuracy of $83.43\%$ than our routing algorithm by a significant margin of $8.68\%$, establishing the effectiveness of our proposed algorithm.

\subsubsection{Effect of the number of instantiation parameters}
The instantiation parameters $D_{cc}$ of the Code Capsule layer acts as the dimensionality of the latent representation of source code. If the dimensionality of the latent representation is higher than required, it can introduce sparsity and/or correlations between the instantiation parameters, reducing the classification accuracy.
On the contrary, if the dimensionality of the latent representation is too low, it may not be sufficient to capture the variations in source code, leading to under-representation, reducing the classification accuracy. Hence, in an attempt to identify a suitable value for $D_{cc}$ for source code classification, we investigate the effect of $D_{cc}$ in the accuracy. As summarized in Table \ref{tab:ablation}, we observed that the most suitable value was $D_{cc}=8$ for the OJ Dataset.
% \yu{Is there any measurement about the training time?}  

\begin{table}[h]
	\caption{Effect of different model variants}
	\label{tab:ablation}
	\begin{center}
		% \begin{adjustbox}{width=1\linewidth}
		\begin{tabular}{|l|c|c|}
			\hline
			\textbf{Model Variant}  & \textbf{Accuracy}  \\
			\hline\hline
			%\dl{Are the numbers really accuracy, precision, F1, or something else?}
			%\dl{Why accuracy is picked as the evaluation metric? If the data is inbalanced, accuracy may not be the best metric.}
			Variable-to-Static Routing Algorithm $\rightarrow$ Dynamic Pooling &  $83.43\%$ \\
			Instantiation parameters $\rightarrow$  $D_{cc} = 4$ &  $90.90\%$ \\
			\hspace{38mm} $D_{cc} = 8$ &  $92.10\%$ \\
			\hspace{38mm} $D_{cc} = 12$ &  $90.33\%$ \\
			\hspace{38mm} $D_{cc} = 16$ &  $91.51\%$ \\
			
			\hline
			TreeCaps with Variable-to-Static Routing and $D_{cc} = 8$ &  $92.11\%$ \\
			
			\hline
		\end{tabular}
		% \end{adjustbox}
	\end{center}
\end{table}
% \yu{Why $D_cc$=16 > $D_cc$=12? Looks like it is not monotonic here?}
% \yu{Why 92.11\% is only slightly better than 92.10\%? Can be useful to see whether VtoS also has different performance with different $D_cc$?}
